# Supplementary material for: Learning Linear Policies for Robust Bipedal Locomotion on Terrains with Varying Slopes
Source: arXiv:2104.01662 source file (2021-08-09)
Supplement: Supplementary file 1 [file Appendix.tex]

% \section{Appendix}


% In a trot gait the diagonally opposite legs move in phase while the other two move out of phase. This means that the swing phase and stance phase of the legs last for the same duration. If we assume that the stance phase (the flat portion of the semi-elliptic trajectory) for any leg lasts for the first half of its cycle and the swing phase for the next half cycle, then taking the hip as the origin, we have the $x,y,z$ position of the foot as:
% \begin{align}
%     \text{stance} &: x = 0.5*l\cos{(2\pi(1-\tau))}, \:\:
%     &y = 0, \:\:
%     &z = -h_d, \quad &\tau \in [0, 0.5), \nonumber \\
%     \text{swing} &: x = 0.5*l\cos{(2\pi(1-\tau))}, \:\:
%     &y = 0, \:\:
%     &z = -h_d + f_c\sin{(2\pi(1-\tau))}, \quad &\tau \in [0.5, 1). \nonumber
% \end{align}
% where $l$ is the step-length ($=\mathbf{ab}$ from Fig. \ref{fig:semi_ellipse}), $h_d$ is the desired height along the support plane normal, $f_c$ is the foot clearance and $\tau$ is the time normalized w.r.t. time period $T$ of one cycle. For Stoch 2, $l \leq 0.136m$, $h_d = 0.243m$, $f_c = 0.06m$ and $T = 0.4s$. The semi-elliptical trajectory which lies in the $X$-$Z$ plane is then transformed according to the action by:
% \begin{align}
%     x^\prime = x_s + x \cos(\phi), \quad
%     y^\prime = y_s + x \sin(\phi), \quad
%     z^\prime = z_s + z,
% \end{align}
% where $x^\prime$, $y^\prime$ and $z^\prime$ are the coordinates of the foot in the leg frame of reference after the transformation, $x_s$, $y_s$ and $z_s$ are the shift (given by $\mathbf{O\acute{O}}$ in Fig. \ref{fig:semi_ellipse}) in the three corresponding Cartesian directions as obtained from the controller, and $\phi$ is the yaw rotation of the semi-ellipse (see Fig. \ref{fig:semi_ellipse}). $x',y',z'$ are then represented in the common body frame by appropriate transformations.
